# Supplementary material for: Direct guaranteed lower eigenvalue bounds with optimal a priori convergence rates for the bi-Laplacian
Source: arXiv:2105.01505 source file (2022-03-07)
Supplement: Supplementary file 2 [file header_supplement.tex]

\parindent 0em
\usepackage{hyperref}
\hypersetup{plainpages=false,
            linkcolor=black,
            citecolor=black,
            urlcolor=black,
            colorlinks=true}
            
% UTF-8 input encoding
\usepackage[utf8]{inputenc}

% Page layout formating of koma-script
\usepackage[automark]{scrlayer-scrpage}

% Language support
\usepackage[english]{babel}

% AMSMath package
\usepackage[intlimits]{amsmath}
\usepackage{amsfonts}
\usepackage{amstext}
\usepackage{amsopn}
\usepackage{mathabx}
\usepackage{url}

%% TikZ
\usepackage{tikz}
\usetikzlibrary{calc}
\usetikzlibrary{patterns}
\tikzset{
  nw/.style={pattern=north west lines, line width=0.1pt, pattern color=#1},
  nw/.default=black
}
\tikzset{
  ne/.style={pattern=north east lines,line width=0.1pt, pattern color=#1},
  ne/.default=black
}

\tikzset{
  every picture/.append style={
    line join=round,
    line cap=round,
  }
}
\usepackage{longtable}
% Misc packages
\usepackage{graphicx}
\usepackage[format=plain]{caption}
\usepackage{subfig}
\usepackage{wrapfig}
\usepackage{enumitem}
\usepackage{nicefrac}

% Font for figures
\tikzstyle{every picture}+=[font=\footnotesize]



%% MATHEMATICAL FORMULAS
\usepackage{amsmath,amssymb,mathtools,commath}
\usepackage{cases}
\usepackage[amsmath,hyperref,thmmarks]{ntheorem}
\numberwithin{equation}{section}
\numberwithin{figure}{section}
\numberwithin{table}{section}

%% THEOREM ENVIRONMENTS
% theorems
\makeatletter
\theoremheaderfont{\bfseries\upshape}
\theoremseparator{.}
%\theoremstyle{plain}
\newtheorem{theorem}{Theorem}[section]
\newtheorem{extratheorem}{Theorem 3.\hspace{-.9ex}}
\newtheorem{lemma}{Lemma}[section]
\newtheorem{proposition}{Proposition}[section]
\newtheorem{example}{Example}[section]
\newtheorem{corollary}{Corollary}[section]
%lemmaAppendix
%\newtheorem*{lem*}{Lemma \Alph{section}}
% definitions
\theoremsymbol{}
\theorembodyfont{\upshape}
\newtheorem{definition}{Definition}[section]
\theoremseparator{}
\newtheorem*{condition}{Condition}
\theoremstyle{break}


% remarks
\theoremstyle{plain}
\theoremseparator{.}
\theoremheaderfont{\itshape}
\newtheorem{remark}{Remark}[section]
\newtheorem*{notation}{Notation}
%\renewcommand*{\thetheorem}{\Alph{lemmaAppendix}}
% proof
\theoremstyle{plain}
\theoremseparator{.}
\newtheorem*{proof2}{Proof}
\theoremsymbol{\ensuremath{\Box}}
\newtheorem*{proof}{Proof}
\theoremseparator{}
\newtheorem*{proofof}{Proof of}

%\usepackage[ruled,vlined]{algorithm2e}
%\usepackage{algorithmic}
\usepackage{algorithm}
\usepackage{algpseudocode}

\algrenewcommand\algorithmicrequire{\textbf{Input:}}
\algrenewcommand\algorithmicensure{\textbf{Output:}}
\floatname{algorithm}{Algorithm}

\usepackage{dirtree}
\usepackage{zref}

\usepackage{booktabs}
\renewcommand{\thetable}{\arabic{section}.\arabic{table}}

% perfect bullet
\let\oldbullet\bullet
  \newlength{\raisebulletlen}
  \setbox1=\hbox{$\bullet$}\setbox2=\hbox{\tiny$\bullet$}
  \setlength{\raisebulletlen}{\dimexpr0.5\ht1-0.5\ht2}
  \renewcommand\bullet{\raisebox{\raisebulletlen}{\,\tiny$\oldbullet$}\,}
\captionsetup{font=footnotesize,margin=3ex}
\pgfdeclarepatterninherentlycolored[\hatchColor]{myLines}{\pgfqpoint{-1pt}{-1pt}}{\pgfqpoint{4pt}{4pt}}{\pgfqpoint{3pt}{3pt}}%
{
    \pgfsetfillcolor{\hatchColor!10}
    \pgfpathrectangle{\pgfqpoint{0pt}{0pt}}{\pgfqpoint{3.1pt}{3.1pt}}
    \pgfusepath{fill}
    \pgfsetlinewidth{0.8pt}
    \pgfsetcolor{\hatchColor}
    \pgfpathmoveto{\pgfqpoint{-0.4pt}{-0.4pt}}
    \pgfpathlineto{\pgfqpoint{3.4pt}{3.4pt}}
    \pgfusepath{stroke}
}

\tikzset{
    hatchColor/.store in=\hatchColor, hatchColor=gray
}
\tikzset{slopetriangle/.style={
  bottom color=black!20,
  middle color=black!5,
  top color=white,
  draw=black
}}

% Integral mean
\def\Xint#1{\mathchoice
{\XXint\displaystyle\textstyle{#1}}%
{\XXint\textstyle\scriptstyle{#1}}%
{\XXint\scriptstyle\scriptscriptstyle{#1}}%
{\XXint\scriptscriptstyle\scriptscriptstyle{#1}}%
\!\int}
\def\XXint#1#2#3{{\setbox0=\hbox{$#1{#2#3}{\int}$}
\vcenter{\hbox{$#2#3$}}\kern-.5\wd0}}
\newcommand{\intmean}{\Xint-}
%%


%listings 
\definecolor{dkgreen}{rgb}{0,0.6,0}
\definecolor{gray}{rgb}{0.5,0.5,0.5}
\definecolor{mauve}{rgb}{0.58,0,0.82}
\usepackage{listings}
\lstset{ %
  language=Matlab,
  basicstyle=\scriptsize\ttfamily,
  keywordstyle=\color{blue},
  deletekeywords={sign},
  commentstyle=\color{dkgreen},
  stringstyle=\color{mauve},
  numberstyle=\color{orange},
  numbers=left,
  numberstyle=\tiny\color{gray},
  stepnumber=1,
  numbersep=5pt,
  backgroundcolor=\color{white},
  showspaces=false,
  showstringspaces=false,
  showtabs=false,
  tabsize=2,
  captionpos=b,
  breaklines=true,
  breakatwhitespace=false,
  belowskip=0pt plus 2pt minus 2pt,
  emph={parfor, ones, repmat, permute, ones},
  emphstyle=\color{blue}
}
\lstdefinestyle{fullsrcsmall}{
  basicstyle=\small\ttfamily,
  xleftmargin=1em,
}
\lstdefinestyle{fullsrcfnsize}{
  basicstyle=\footnotesize\ttfamily,
  xleftmargin=2em,
}
\lstdefinestyle{fullsrcscsize}{
  basicstyle=\scriptsize\ttfamily,
  numbers=none,
  xleftmargin=2em,
}
\lstdefinestyle{inline}{
  basicstyle=\ttfamily,
  numbers=none,
  xleftmargin=0em,
}
\lstdefinestyle{inlinesmall}{
  basicstyle=\small\ttfamily,
  numbers=none,
  xleftmargin=0em,
}
\lstdefinestyle{inlinefnsize}{
  basicstyle=\footnotesize\ttfamily,
  numbers=none,
  xleftmargin=1em,
}
